# Supplementary material for: Recursion of Thought: A Divide-and-Conquer Approach to Multi-Context Reasoning with Language Models
Source: arXiv:2306.06891 source file (2023-06-12)
Supplement: Supplementary file 10 [file appendix_rot_alg.tex]

\documentclass[../acl2023_rot.tex]{subfiles}

\begin{document}

\section{RoT Inference Algorithm}
\label{sec:rot_alg}

\begin{algorithm}[H]
  \caption{Recursion of Thought Inference}
  \label{alg:rot}
  \begin{algorithmic}[1]
    \Require{A sequence model $\mathcal M$ trained for Recursion of Thought, a question sequence $Q$}
    \Function{RoT}{$\mathcal M$, $Q$} \label{alg:rot:start}
    \State $X \gets Q$ \Comment{Initialize context with $Q$}
    \State $i_\mathrm{ans} \gets |X|+1$ \Comment{Start of answer}
    \State $t \gets false$  \Comment{Tail recursion}
    \While{True}
    \State $x \gets \mathcal M(X)$ \Comment{Generate next token}
    \State $X \gets $ $[X; x]$
    %			\State $x \gets Xx$ \Comment{Append $x$ to context}
    \If{$x = \STOP$}
    \State \Return $X_{i_\mathrm{ans}:|X|}$ \label{alg:rot:return}
    \ElsIf{$x = \GO$}
    \State $i_{\mathrm{go}} \gets |X|$ \Comment{Mark last \GO} \label{alg:rot:go}
    \ElsIf{$x = \TAIL$}
    \State $i_{\mathrm{go}} \gets |X|$
    \State $t \gets true$ \label{alg:rot:mark_tail} \Comment{Mark tail recursion}
    \ElsIf{$x = \THINK$}
    \State $Q^\mathrm{sub} \gets X_{i_{\mathrm{go}}: |X|-1}$ \label{alg:rot:q_sub}
    \State $A^\mathrm{sub} \gets \Call{RoT}{\mathcal M, Q^\mathrm{sub}}$ \label{alg:rot:call}
    \If{$t$}
    \State \Return $A^\mathrm{sub}$ \label{alg:rot:return_tail}
    \EndIf
    \State $X \gets [X_{1:|X|-1}; A^\mathrm{sub}]$ \label{alg:rot:replace}
    \State \Comment{Replace \THINK with $A^{\mathrm{sub}}$}
    \State $i_{\mathrm{ans}} \gets |X|+1$ \label{alg:rot:i_ans}
    \EndIf
    \EndWhile
    \EndFunction
  \end{algorithmic}
\end{algorithm}

\end{document}
