# Supplementary material for: Recursion of Thought: A Divide-and-Conquer Approach to Multi-Context Reasoning with Language Models
Source: arXiv:2306.06891 source file (2023-06-12)
Supplement: Supplementary file 12 [file appendix_target_seq.tex]

\documentclass[../acl2023_rot.tex]{subfiles}

\begin{document}
\section{Target Sequence}
\label{sec:target_seq}

\begin{algorithm}[H]
  \caption{Creating the target sequence}
  \label{alg:context_conversion}
  \begin{algorithmic}[1]
    \Require Context $X=[Q; Q^{\mathrm{sub},1}; A^{\mathrm{sub},1}; \allowbreak \ldots; Q^{\mathrm{sub},N}; A^{\mathrm{sub},N}; A]$
    %		\State $X \gets Q$ \label{alg:ctx:x-init}
    \State $Y \gets \underbrace{\PAD ... \PAD}_{|Q|}$ \label{alg:ctx:q}
%				\For{$(Q^{\mathrm{sub},n}, A^{\mathrm{sub},n})
%					\hspace{-1pt} \in \hspace{-1pt}  \{(Q^{\mathrm{sub},*}, A^{\mathrm{sub},*})\}$} \label{alg:ctx:sub_start}
    \For{$n$ in $1...N$}
    %		\State $X \gets X + Q^{\mathrm{sub},n} + A^{\mathrm{sub},n}$
    \State $Y \gets [Y; Q^{\mathrm{sub},n}]$
    \State $Y \gets [Y; \THINK\underbrace{\PAD ... \PAD}_{|A^{\mathrm{sub},n}| - 1}]$ \label{alg:ctx:y-a-sub}
    %		\State \Comment{Instead of $A^{\mathrm{sub},n}$}
    \EndFor \label{alg:ctx:sub_end}
    %		\State $X \gets X + A_{1: |A| - 1}$
    \State $Y \gets [Y; A]$ \label{alg:ctx:a}
    \State \Return $Y$
  \end{algorithmic}
\end{algorithm}

\begin{figure*}[h]
  \centering
	\includegraphics[width=0.9\textwidth, trim={0 22.8cm 0 0}, clip]{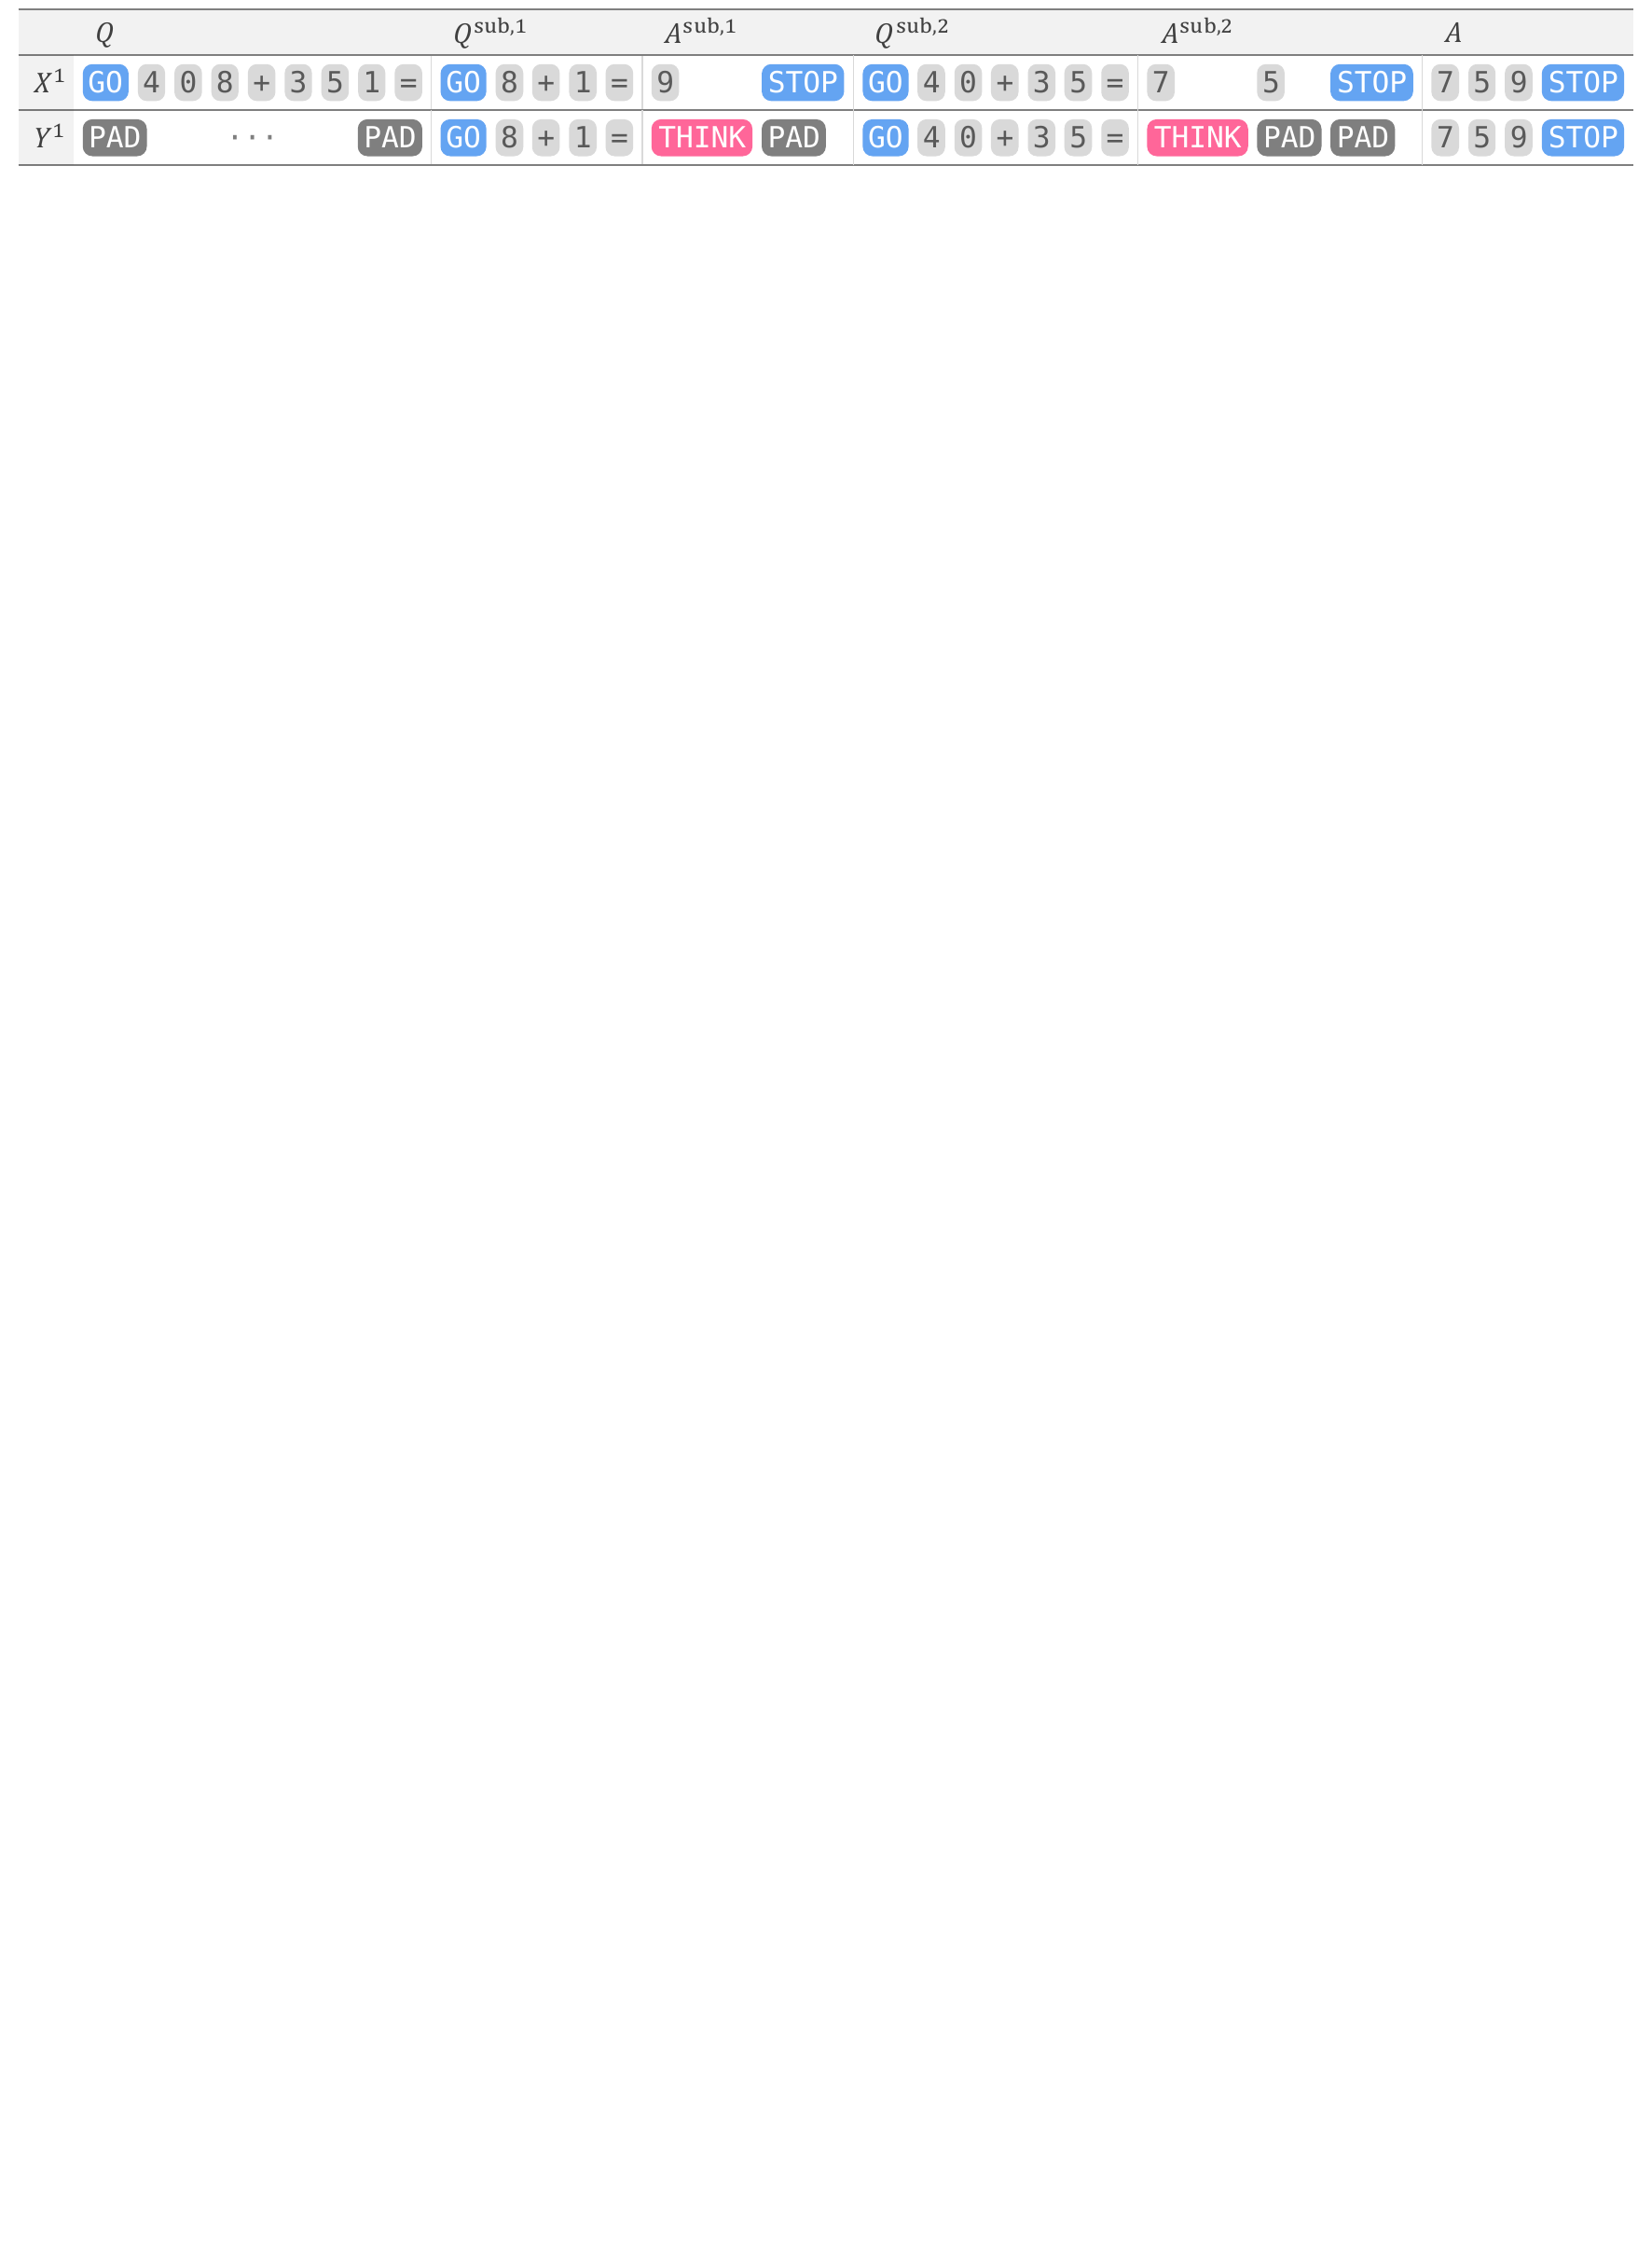}
	% \vspace{-5mm}
	\caption{
		The target sequence $Y^1$ for $X^1$ in Figure \ref{fig:rot}.
	}
	\label{fig:target}
\end{figure*}

\end{document}
